# Supplementary material for: Programming Strategies for Irregular Algorithms on the Emu Chick
Source: arXiv:1901.02775 source file (2018-12-03)
Supplement: Supplementary file 1 [file ad-appendix.tex]

% LaTeX template for the Supercomputing Conference series Artifact Description (AD) appendix  
% V20180131
% (C)opyright 2018

% Derived with permission by Michael Heroux (Sandia National Laboratories, St. John's University, MN)
% from ae-20160509.tex 
% written by Grigori Fursin (cTuning foundation, France and dividiti, UK) 
% and Bruce Childers (University of Pittsburgh, USA)
% (C)opyright 2014-2016

% acmart is available at https://www.acm.org/publications/proceedings-template
%\documentclass[sigconf,twocolumn]{acmart}
% IEEETrans is available at https://www.ieee.org/conferences_events/conferences/publishing/templates.html
%\documentclass{IEEETran}
%\begin{document}

%\special{papersize=8.5in,11in}

%\appendix

%%%%%%%%%%%%%%%%%%%%%%%%%%%%%%%%%%%%%%%%%%%%%%%%%%%%
% When adding this appendix to your paper, 
% please remove above part
%%%%%%%%%%%%%%%%%%%%%%%%%%%%%%%%%%%%%%%%%%%%%%%%%%%%

\section{Artifact Description Appendix:Optimizing Irregular Algorithms for the Emu Chick}

%%%%%%%%%%%%%%%%%%%%%%%%%%%%%%%%%%%%%%%%%%%%%%%%%%%%%%%%%%%%%%%%%%%%%
\subsection{Abstract}

This appendix details the three different application kernels that were evaluated in this paper how they can be run on the Emu Chick prototype hardware. Note that hardware access is currently limited to
users via the Emu DRIVE program for developers. %\url{http://www.emutechnology.com/software/drive-program/}.

%%%%%%%%%%%%%%%%%%%%%%%%%%%%%%%%%%%%%%%%%%%%%%%%%%%%%%%%%%%%%%%%%%%%%
\subsection{Description}

\subsubsection{Check-list (artifact meta information)}

{\small
\begin{itemize}
  \item {\bf Algorithms: SpMV, BFS, and gsaNA}
  \item {\bf Compilation: Compile using the included Makefiles.}
  \item {\bf Binaries: csr\_spmv.mwx, dynograph.mwx, gsana.mwx}
  \item {\bf Data sets: See below for each algorithm}
  \item {\bf Hardware: The Emu Chick platform with a specific NCDIMM (2.1.7), system software (1.4), and stationary core code (2.0.32). Changes or updates to any of this ``firmware'' will likely change the results.}
  \item {\bf Execution: The same executable can be run on the simulator or hardware using either \inlinecode{Bash}{emusim.x} or \inlinecode{Bash}{emu_handler_and_loader} on the hardware}
  \item {\bf Output: The algorithms generate time to run. Python and Python-based notebooks are used to convert to effective bandwidth or MTEPS based on input type and size}
  \item {\bf Experiment workflow: See below section.}
  \item {\bf Experiment customization: When compiling you can use the \inlinecode{Bash}{-DREPLICATE_X} flag to specify whether X is replicated}
  \item {\bf Publicly available?: Yes} \\
\end{itemize}

\subsubsection{How software can be obtained}
The experiments in this paper can be reproduced using the code in the Github repo located at: \textit{removed for blind review}
The Emu compiler and 18.02 software stack can be accessed by logging on to the Emu Chick prototype system through the Emu DRIVE program. \\

%https://github.com/hpcgarage/emuapps\_sc18

\subsubsection{Hardware dependencies}
Replication of the experiments in this paper requires the use of the Emu Chick prototype hardware with a firmware of 1.0 or greater. Note that newer revisions of the base FPGA or ``NCDIMM'' hardware may result in different performance results. \\ 

\subsubsection{Software dependencies}
Experiments in this paper depend primarily on the use of the Emu C-based compiler tools and the Emu execution environment. Python is used for analysis of output data.

\subsubsection{Datasets}

\begin{itemize}
\item Sparse matrix inputs include: 

\begin{itemize}
\item synthetic Laplacians generated inputs that are created corresponding to a $d$-dimensional $k$-point stencil on a grid of length $n$ in each dimension. For the tested synthetic matrices, $d=2$ and $k=5$, resulting in a $n^2 \times n^2$ Laplacian with five diagonals. 
\item Real-world sparse matrices obtained from the SuiteSparse (formerly UF) sparse matrix collection (see Table \ref{table:spmv-real}). 
\end{itemize}

\item Both versions of BFS application (i.e., one using thread migrations and another using remote writes) inputs include
\begin{itemize}
\item RMAT graph specified by Graph500 and (Erd\"os-R\'enyi) graph 
\item The input sizes of both graph graphs are varied using the parameter {\tt scale}\footnote{A scale of 1 for an input graph refers to having 4K vertices.} from 8 to 17.
\end{itemize}
\item {\sc gsaNA} uses different DBLP graphs: 
\begin{itemize}
\item DBLP~\cite{ref:dblp-site} graphs from years
$2015$ and $2017$ that are created in~\cite{yasar2018iterative} are used.
Two graphs have nearly $48K$, $59K$ vertices and $453K$, $656K$ edges
respectively.
\item From $2^9$ to $2^{15}$ number of vertices and their intra edges are filtered from these two graphs and seven different graph pairs are generated.
\end{itemize}
\end{itemize}

%%%%%%%%%%%%%%%%%%%%%%%%%%%%%%%%%%%%%%%%%%%%%%%%%%%%%%%%%%%%%%%%%%%%%
\subsection{Installation}

All of the three application kernels can be accessed from a sub-folder in the provided repository and built on a node with the Emu compiler tools using the specific compilation instructions and Makefiles.
%\textbf{SpMV:} Each of the application kernels can be accessed from a sub-folder in the provided repo and built on a node with the Emu compiler tools using the specific compilation instructions and Makefiles.

%\TODO{G500:}

%\textbf{{\sc gsaNA}:} Source-code for similarity computation can be 
%accessed from a sub-folder in the provided repo and built on a node 
%with the Emu compiler tools using the specific compilation instructions 
%and Makefile.

%%%%%%%%%%%%%%%%%%%%%%%%%%%%%%%%%%%%%%%%%%%%%%%%%%%%%%%%%%%%%%%%%%%%%
\subsection{Experiment workflow}
In many cases, the code will be compiled on a host node and then the binary and input dataset will be simulated on the host node or copied to a hardware node. 

%For SpMV: 
%\begin{enumerate}
% \item Compile the application
% \item Simulate the application using the \inlinecode{Bash}{emusim.x} command on %the host with synthetic or real-world data sets
% \item scp the bin/ and data/ directories to an Emu node
% \item Execute the same binary on the Emu node using the \inlinecode{Bash}{emu\_handler\_and\_loader} command
% \item Parameters for running the SpMV binary are as follows: 
% \begin{lstlisting}[language=Bash, backgroundcolor = \color{lightgray}]
%emu_handler_and_loader 0 0 csr_spmv.mwx 
%<mtx_file/synth> <0/matrix_size> <data_layout=0,1,2> %<serial_spawn/recursive_spawn=0/1> <nthreads>
% \end{lstlisting}
%\end{enumerate}

\begin{enumerate}
 \item Compilation -- Use the provided {\tt cmake} files
 \item Running on a simulator -- Run using the \inlinecode{Bash}{emusim.x} command on the compiled code from the previous step on a host machine
 \item Running on the hardware -- After copying the bin/ and data/ directories to an Emu node, execute the compiled code on the Emu node using the \inlinecode{Bash}{emu\_handler\_and\_loader} command
 \item The parameters for running the applications are as follows:
 \begin{itemize}
 	\item SpMV  
     \begin{lstlisting}[language=Bash, backgroundcolor = \color{lightgray}]
emu_handler_and_loader 0 0 -- csr_spmv.mwx 
<mtx_file/synth> <0/matrix_size> <data_layout=0,1,2> <serial_spawn/recursive_spawn=0/1> <nthreads>
 \end{lstlisting}
 	\item BFS 
         \begin{lstlisting}[language=Bash, backgroundcolor = \color{lightgray}]
emu_handler_and_loader 0 0 -- dynograph.mwx --graph500 <scale>
 \end{lstlisting}
 \item gsaNA
  \begin{lstlisting}[language=Bash, backgroundcolor = \color{lightgray}]
emu_handler_and_loader 0 0 -- gsana.mwx 
<graph_number> <layout_type=0,1> <computation_type=0,1> <number_of_threads>
 \end{lstlisting}
 \end{itemize}
\end{enumerate}

%For gsaNA:
%\begin{enumerate}
% \item Compile the application ({\tt make})
% \item Simulate the application using the \inlinecode{Bash}{emusim.x} command on the host with a graph
% \item scp the bin/ and data/ directories to an Emu node
% \item Execute the same binary on the Emu node using the \inlinecode{Bash}{emu\_handler\_and\_loader} command
% \item Parameters for running the {\sc gsaNA} binary are as follows: 
 %\begin{lstlisting}[language=Bash, backgroundcolor = \color{lightgray}]
%emu_handler_and_loader 0 0 gsana.mwx 
%<graph_number> <layout_type=0,1> <computation_type=0,1> <number_of_threads>
 %\end{lstlisting}
%\end{enumerate}

%%%%%%%%%%%%%%%%%%%%%%%%%%%%%%%%%%%%%%%%%%%%%%%%%%%%%%%%%%%%%%%%%%%%%
\subsection{Evaluation and expected result}

Each application kernel presents its outputs in a specific fashion related to its purpose. SpMV and gsaNA
produce output that relates to overall memory bandwidth (data transferred) while Graph 500 BFS uses a more
traditional TEPS number that is standard for Graph500 implementations. 

On the prototype hardware we expect that results should be somewhat deterministic when experiments are repeated. This is because performance variance is typically related to thread migration as opposed to caching effects on traditional architectures. Simulation results take a long time to generate due to cycle-accurate simulation slowdowns, but previous work and our experiments show that simulation output matches relatively closely to hardware, with the exception of thread spawn limits (which can cause crashes on the hardware) and thread buffering limits that exist on the hardware but not in simulation.  

%%%%%%%%%%%%%%%%%%%%%%%%%%%%%%%%%%%%%%%%%%%%%%%%%%%%%%%%%%%%%%%%%%%%%
\subsection{Experiment customization}
Other than parameter sweeps, each application may have a specific set of parameters to test different variants of the experiment. For example, with gsaNA, thread count can be varied, blocking type can be changed and ALL or PAIR similarity comparisons can be used for neighboring buckets. Each benchmark provides a script that demonstrates the different parameter sweeps for a specific experiment.

%%%%%%%%%%%%%%%%%%%%%%%%%%%%%%%%%%%%%%%%%%%%%%%%%%%%%%%%%%%%%%%%%%%%%
%\subsection{Notes}
