# Supplementary material for: Programming Strategies for Irregular Algorithms on the Emu Chick
Source: arXiv:1901.02775 source file (2018-12-03)
Supplement: Supplementary file 2 [file ae-appendix.tex]

% LaTeX template for the Supercomputing Conference series Computational Results Analysis (CRA) appendix  
% V20180131
% (C)opyright 2018

% Derived with permission by Michael Heroux (Sandia National Laboratories, St. John's University, MN)
% from ae-20160509.tex 
% written by Grigori Fursin (cTuning foundation, France and dividiti, UK) 
% and Bruce Childers (University of Pittsburgh, USA)
% (C)opyright 2014-2016

% acmart is available at https://www.acm.org/publications/proceedings-template
%\documentclass[sigconf,twocolumn]{acmart}
% IEEETrans is available at https://www.ieee.org/conferences_events/conferences/publishing/templates.html

\section{Trust Appendix: Lessons Learned For Irregular Algorithms on the Emu Chick}

%%%%%%%%%%%%%%%%%%%%%%%%%%%%%%%%%%%%%%%%%%%%%%%%%%%%%%%%%%%%%%%%%%%%%
\subsection{Abstract}

{\em
Overall description of your approach and how trustworthiness of your results is improved.
For example: How you validated timers, what manufactured solution or spectral properties you leveraged, etc.}

{\em If a paper has no computational results and submits this appendix, the authors only need to complete this abstract subsection and mention that the paper has no computational results.  Other subsections can be removed.}

%%%%%%%%%%%%%%%%%%%%%%%%%%%%%%%%%%%%%%%%%%%%%%%%%%%%%%%%%%%%%%%%%%%%%

\subsection{Results Analysis Discussion}

{\em Description of results, their correctness and any concerns about them. If your paper is only about performance, describe how you assure the quality of performance measurements and that you have preserved correct computational results.}

For SpMV, performance should be between pointer chasing and the "peak" bandwidth of 1.2 GB/s.

%%%%%%%%%%%%%%%%%%%%%%%%%%%%%%%%%%%%%%%%%%%%%%%%%%%%%%%%%%%%%%%%%%%%%
\subsection{Summary}

{\em Final summary demonstrating the trustworthiness of your results.}

%%%%%%%%%%%%%%%%%%%%%%%%%%%%%%%%%%%%%%%%%%%%%%%%%%%%%%%%%%%%%%%%%%%%%
\subsection{Notes}
